# Supplementary material for: Guiding Human-Object Interactions with Rich Geometry and Relations
Source: arXiv:2503.20172 source file (2025-03-26)
Supplement: Supplementary file 1 [file ref_appendix.tex]

\begin{thebibliography}{26}\itemsep=-1pt
\bibitem{guochuan}\label{47}
C. Guo, S. Zou, X. Zuo, S. Wang, W. Ji, X. Li, L. Cheng. Generating diverse and natural 3D human motions from text. In {\it CVPR}, 2022.

\bibitem{licontrollable}\label{48}
J. Li, A. Clegg, R. Mottaghi, J. Wu, X. Puig, C. Liu. Controllable human-object interaction synthesis. In {\it{ECCV}}, 2024.

\bibitem{liobject}\label{49}
J. Li, J. Wu, C. Liu. Object Motion Guided Human Motion Synthesis. In {\it{ACM TOG}}, 2023.

\bibitem{fanarctic}\label{50}
Z. Fan, O. Taheri, D. Tzionas, M. Kocabas, M. Kaufmann, M. Black, O. Hilliges. {ARCTIC}: A Dataset for Dexterous Bimanual Hand-Object Manipulation. In {\it{CVPR}}, 2023.

\bibitem{vdt}\label{51}
H. Lu, G. Yang, N. Fei, Y. Huo, Z. Lu, P. Luo, M. Ding. Vdt: General-purpose video diffusion transformers via mask modeling. In arXiv:2305.13311, 2023.

\bibitem{mdm}\label{52}
G. Tevet, S. Raab, B. Gordon, Y. Shafir, A. Bermano, D. Cohen-Or. Human Motion Diffusion Model. In {\it{ICLR}}, 2023.

\bibitem{peng2023hoi}
X. Peng, Y. Xie, Z. Wu, V. Jampani, D. Sun, H. Jiang. Hoi-diff: Text-driven synthesis of 3d human-object interactions using diffusion models. In arXiv:2312.06553, 2023.

\bibitem{diller2024cg}
C. Diller, A. Dai. Cg-hoi: Contact-guided 3d human-object interaction generation. In {\it{CVPR}}, 2024.


% \bibitem{kim2024parahome}
% J. Kim, J. Kim, J. Na, H. Joo. ParaHome: Parameterizing Everyday Home Activities Towards 3D Generative Modeling of Human-Object Interactions. In arXiv:2401.10232, 2024.

\end{thebibliography}
